# Supplementary material for: AIMY: An Open-source Table Tennis Ball Launcher for Versatile and High-fidelity Trajectory Generation
Source: arXiv:2210.06048 source file (2023-03-17)
Supplement: Supplementary file 1 [file launcher_speed_comp.tex]

\begin{table}[H]
\centering
\caption{Speed and Topspin comparison of the table tennis ball launchers}
\label{tab:my-table}
\begin{tabular}{@{}ccc@{}}
\toprule
\textbf{Ball Launcher} & \textbf{Max. Speed [\SI{\meter\per\second}]} & \textbf{Max. Topspin [\per\second]} \\ \midrule
TTmatic 303A & 9.8 & 64.0 \\
Power-Pong 2050 & 10.7 & 106.7 \\
AIMY v2 & 15.4 & 192.0 \\ \bottomrule
\end{tabular}
\end{table}
